# Supplementary material for: Fingerprints of Mott and Slater gaps in the core-level photoemission spectra of antiferromagnetic iridates
Source: arXiv:2404.12646 source file (2025-10-06)
Supplement: Supplementary file 1 [file sm.tex]

\documentclass[reprint,twocolumn,superscriptaddress,secnumarabic,amssymb, nobibnotes, aps,pra]{revtex4-2}

% Some other (several out of many) possibilities
%\documentclass[eqsecnum,aps,draft]{revtex4-2}
%\documentclass[prb]{revtex4}% Physical Review B
%\documentclass[twocolumn,showpacs,prb]{revtex4-2}
%\documentclass[twocolumn,showpacs,prb]{revtex4-2}% Physical Review B
%\documentclass[twocolumn,superscriptaddress,showpacs,prb]{revtex4-2}% Physical Review B

\usepackage{graphicx}%
\usepackage{dcolumn}
\usepackage{amsmath}
\usepackage{amssymb}
\usepackage{bm}
\usepackage{color}
\usepackage[whole]{bxcjkjatype}
\usepackage{xspace}
\usepackage{comment}

\def\sroa{Sr$_{2}$IrO$_{4}$\xspace}
\def\srob{Sr$_{3}$Ir$_{2}$O$_{7}$\xspace}

%\nofiles
\begin{document}

\newcommand{\Add}[1]{\textcolor{red}{#1}}
\newcommand{\Erase}[1]{\textcolor{red}{\sout{\textcolor{black}{#1}}}}

\renewcommand{\figurename}{FIG.~S\!\!}
\renewcommand{\tablename}{TABLE~S\!\!}
\newcommand{\tc}[2]{\textcolor{#1}{#2}}

%\preprint{HEP/123-qed}

%%%%%%%%%%%%%%%%%*Title*%%%%%%%%%%%%%%%%%%%

\preprint{submitted to Physical Review Letters}

\title{Supplemental Material: Fingerprints of Mott and Slater gaps in the core-level photoemission spectra of antiferromagnetic iridates}

\author{K. Nakagawa}
\affiliation{Graduate School of Natural Science, Konan University, Kobe 658-8501, Japan }
\affiliation{RIKEN SPring-8 Center, Sayo, Hyogo 679-5148, Japan}

\author{A. Hariki}
\affiliation{Graduate School of Engineering, Osaka Prefecture University, Sakai, Osaka 599-8531, Japan}
\affiliation{Graduate School of Engineering, Osaka Metropolitan University, Sakai, Osaka 599-8531, Japan}

\author{T. Okauchi}
\affiliation{Graduate School of Engineering, Osaka Metropolitan University, Sakai, Osaka 599-8531, Japan}

\author{H. Fujiwara}
\affiliation{RIKEN SPring-8 Center, Sayo, Hyogo 679-5148, Japan}
\affiliation{Graduate School of Engineering Science, The University of Osaka, Toyonaka, Osaka 560-8531, Japan}
\affiliation{
Spintronics Research Network Division, 
Institute for Open and Transdisciplinary Research Initiatives,
The University of Osaka, 
Suita, Osaka 565-0871, Japan}

\author{K.-H. Ahn}   % ORCID 0000-0001-8188-8926
\affiliation{Institute of Physics, Czech Academy of Sciences, Cukrovarnick\'{a} 10, 162 00 Praha 6, Czechia}

\author{Y. Murakami}
\affiliation{Graduate School of Natural Science, Konan University, Kobe 658-8501, Japan }
\affiliation{RIKEN SPring-8 Center, Sayo, Hyogo 679-5148, Japan}

\author{S.~Hamamoto}
\affiliation{RIKEN SPring-8 Center, Sayo, Hyogo 679-5148, Japan}

\author{Y. Kanai-Nakata}
\author{T. Kadono}
\affiliation{RIKEN SPring-8 Center, Sayo, Hyogo 679-5148, Japan}
\affiliation{College of Science and Engineering, Ritsumeikan University, Kusatsu, Shiga 525-8577, Japan}

\author{A. Higashiya}
\affiliation{RIKEN SPring-8 Center, Sayo, Hyogo 679-5148, Japan}
\affiliation{Faculty of Science and Engineering, Setsunan University, Neyagawa, Osaka 572-8508, Japan}

\author{K. Tamasaku}
\author{M.~Yabashi}
\author{T. Ishikawa}
\affiliation{RIKEN SPring-8 Center, Sayo, Hyogo 679-5148, Japan}

\author{A. Sekiyama}
\affiliation{RIKEN SPring-8 Center, Sayo, Hyogo 679-5148, Japan}
\affiliation{Graduate School of Engineering Science, The University of Osaka, Toyonaka, Osaka 560-8531, Japan}
\affiliation{
Spintronics Research Network Division, 
Institute for Open and Transdisciplinary Research Initiatives,
The University of Osaka, 
Suita, Osaka 565-0871, Japan}

\author{S. Imada}
\affiliation{RIKEN SPring-8 Center, Sayo, Hyogo 679-5148, Japan}
\affiliation{College of Science and Engineering, Ritsumeikan University, Kusatsu, Shiga 525-8577, Japan}

\author{J. Kune\v{s}}
\affiliation{Institute of Solid State Physics, TU Wien, 1040 Vienna, Austria}
\affiliation{Department of Condensed Matter Physics, Faculty of
  Science, Masaryk University, Kotl\'a\v{r}sk\'a 2, 611 37 Brno,
  Czechia}

\author{K. Takase}
\affiliation{College of Science and Technology, Nihon University, Tokyo 101-8308, Japan}

\author{A. Yamasaki}
\affiliation{RIKEN SPring-8 Center, Sayo, Hyogo 679-5148, Japan}
\affiliation{Faculty of Science and Engineering, Konan University, Kobe 658-8501, Japan }

%\date{\today}

\maketitle

%%%%%%%%%%%%%%%%%%%%%%%%%%%%%%%%%%%%%%%%%%%%%%%%%%%%%%
\onecolumngrid\
\begin{figure*}[htbp]
\includegraphics[width=1.0\columnwidth]{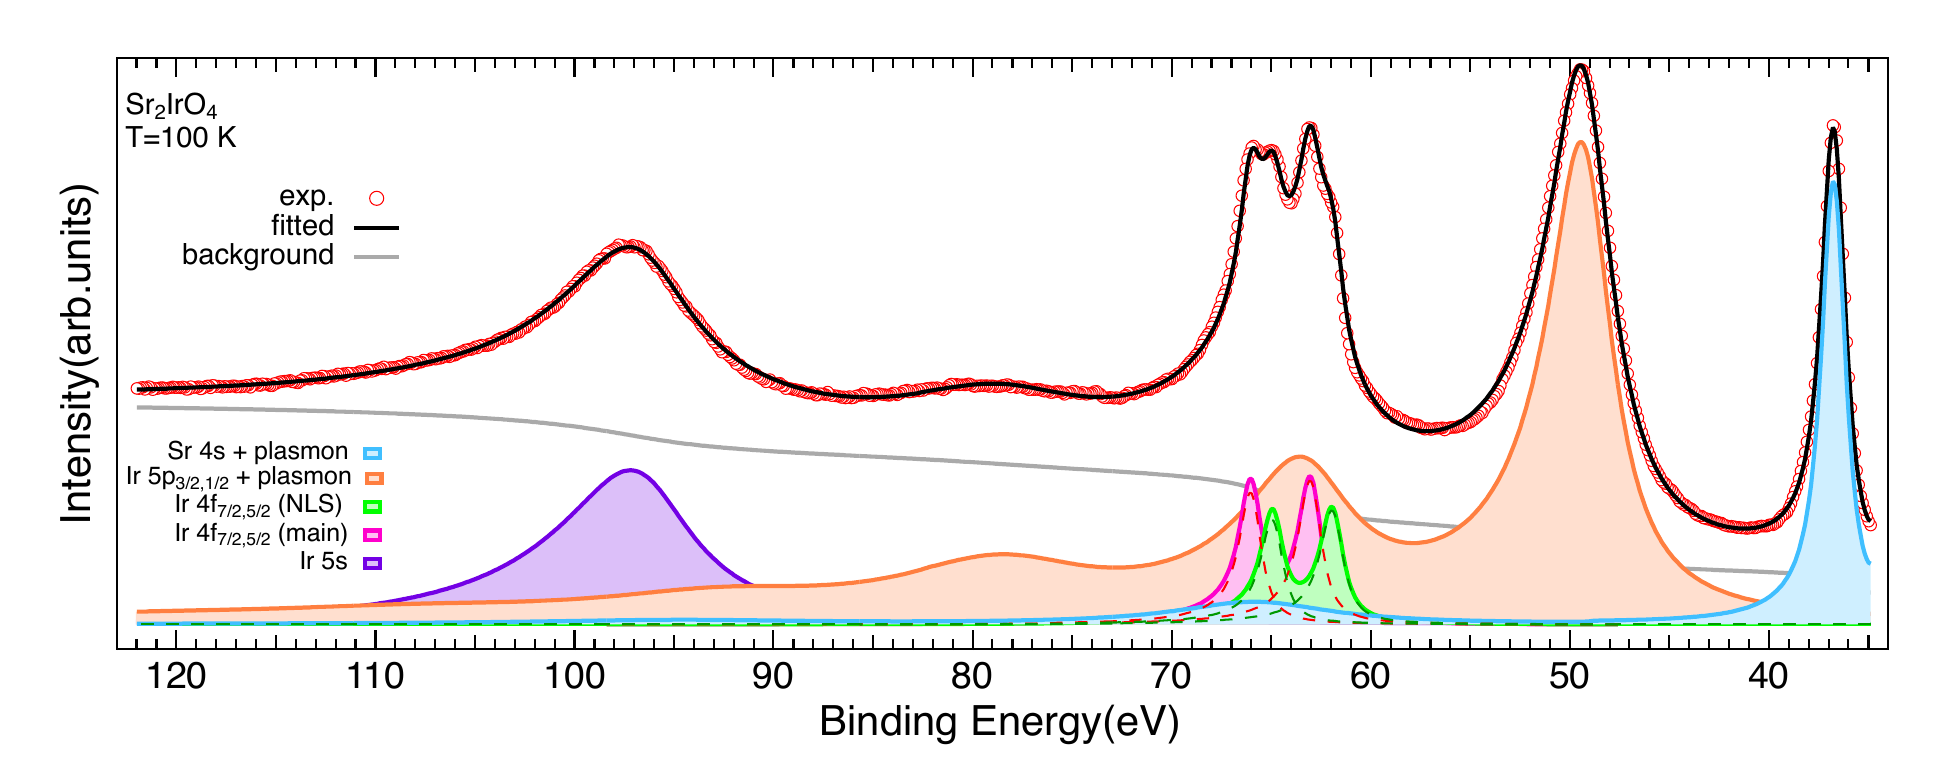}
\caption{
Overview of a general line-shape analysis for Ir core-level HAXPES spectrum of \sroa.
The atomic spin-orbit splitting energies of Ir 5$p$ and 4$f$
core levels are used for the fit. The branching ratio of Ir 5$p_{3/2}$ and 5$p_{1/2}$ 
states is kept at 2:1. The plasmon energy is set to 29.0~eV.
Note that the deconvolved Ir $4f$ spectrum is not used for comparison
with the theoretical spectrum.}
\label{fig_fitting}
\end{figure*}
\twocolumngrid\
%%%%%%%%%%%%%%%%%%%%%%%%%%%%%%%%%%%%%%%%%%%%%%%%%%%%%%

%%%%%%%%%%%%%%%%%%%%%%%%%%%%%%%%%%%%%%%%%%%%%%%%%%%%%%
\twocolumngrid\
\begin{figure*}[htbp]
\includegraphics[width=1.2\columnwidth]{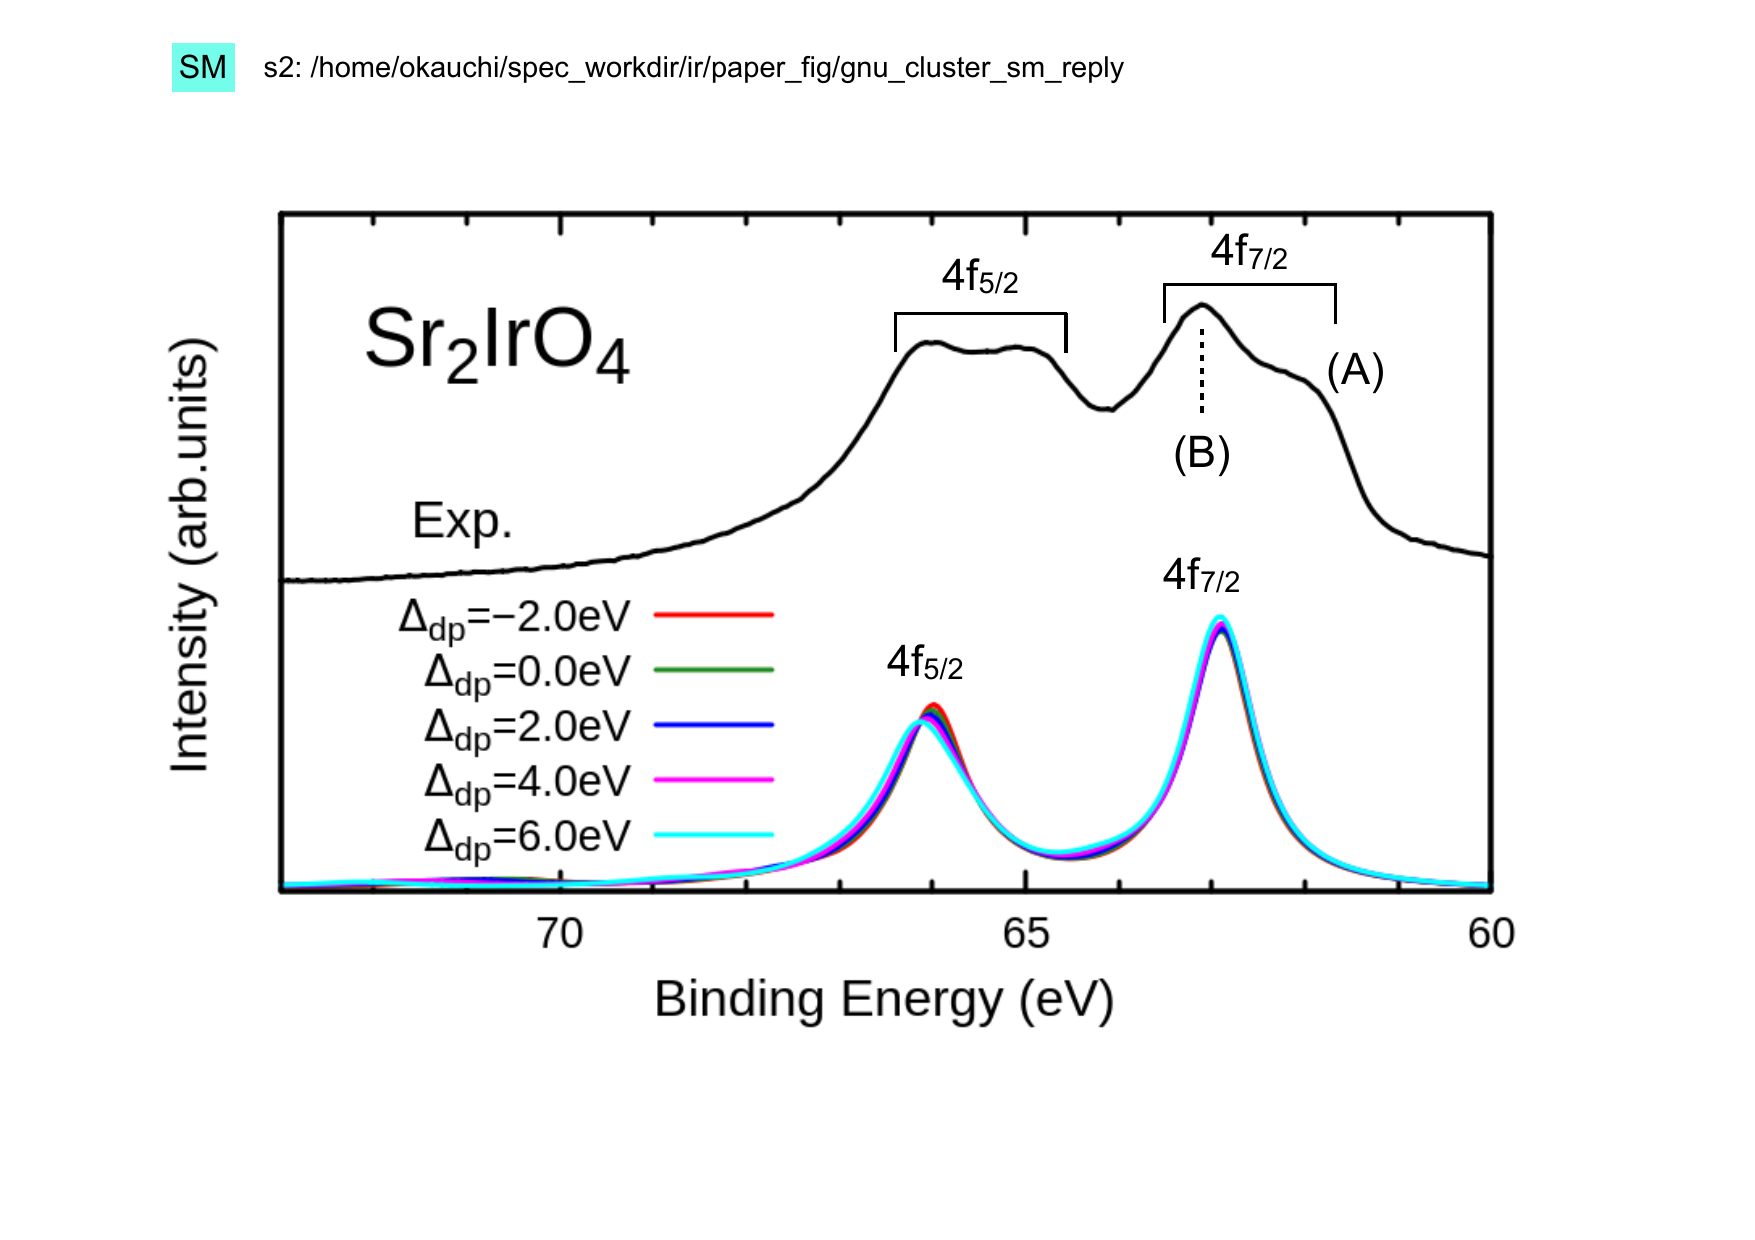}
\caption{Ir 4$f$ XPS spectra of \sroa calculated by the IrO$_6$ cluster model for selected charge-transfer energies $\Delta_{dp}$. The experimental HAXPES spectrum at 100~K is shown for comparison.}
\label{fig_cluster_sm}
\end{figure*}
%%%%%%%%%%%%%%%%%%%%%%%%%%%%%%%%%%%%%%%%%%%%%%%%%%%%%%

%%%%%%%%%%%%%%%%%%%%%%%%%%%%%%%%%%%%%%%%%%%%%%%%%%%%%%
\begin{figure*}[htbp]
\includegraphics[width=1.2\columnwidth]{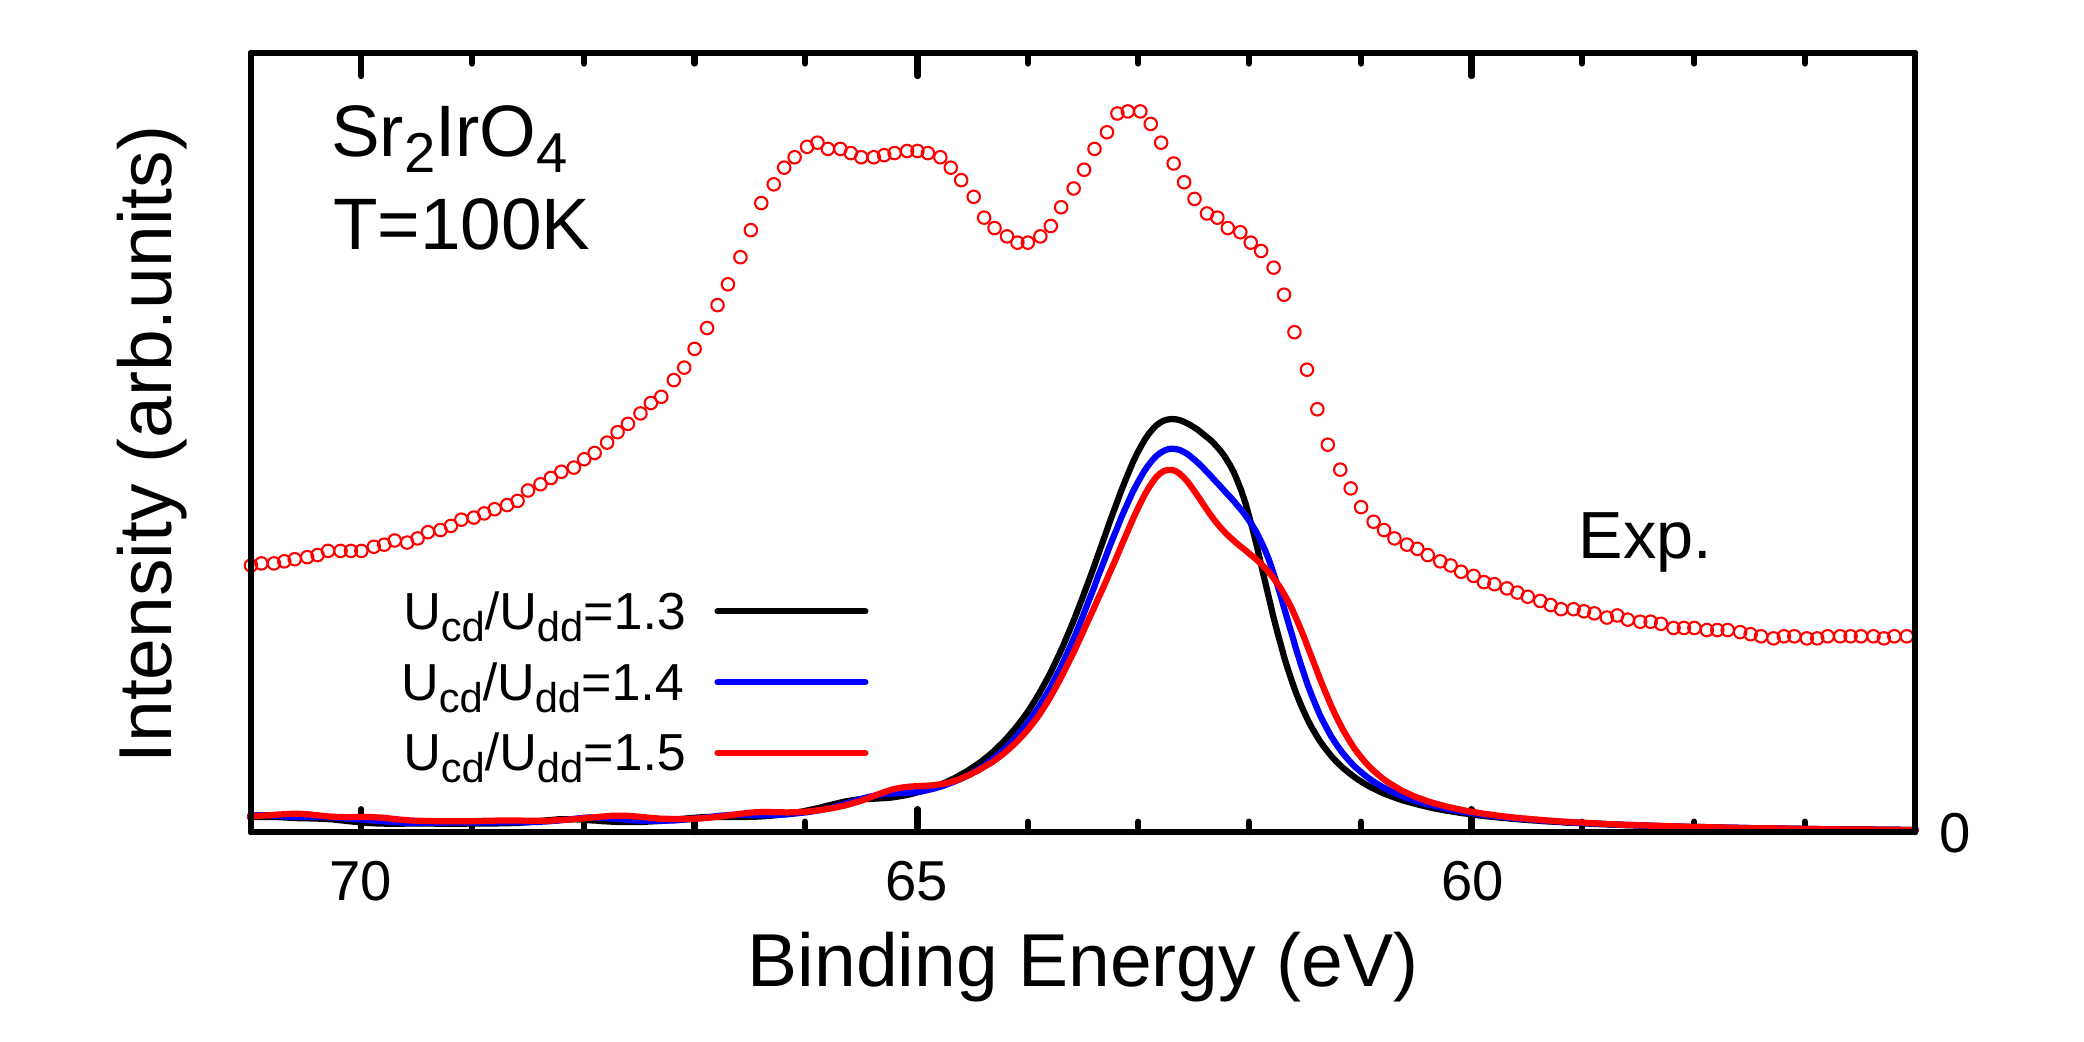}
\caption{Core-level XPS spectra calculated using the LDA+DMFT AIM method for the AFM solution in Sr$_2$IrO$_4$ with different core-hole potential \(U_{cd}\) values. The experimental spectrum is shown for comparison.}
\label{fig_fit_Ir4f}
\end{figure*}

\end{document}
